# Supplementary material for: Should public health policy exempt cases with low viral load from isolation during an epidemic?: a modelling study
Source: arXiv:2412.17428 source file (2025-01-31)

Cumulative infection curves for all 100 simulations under the multiple tests scenario

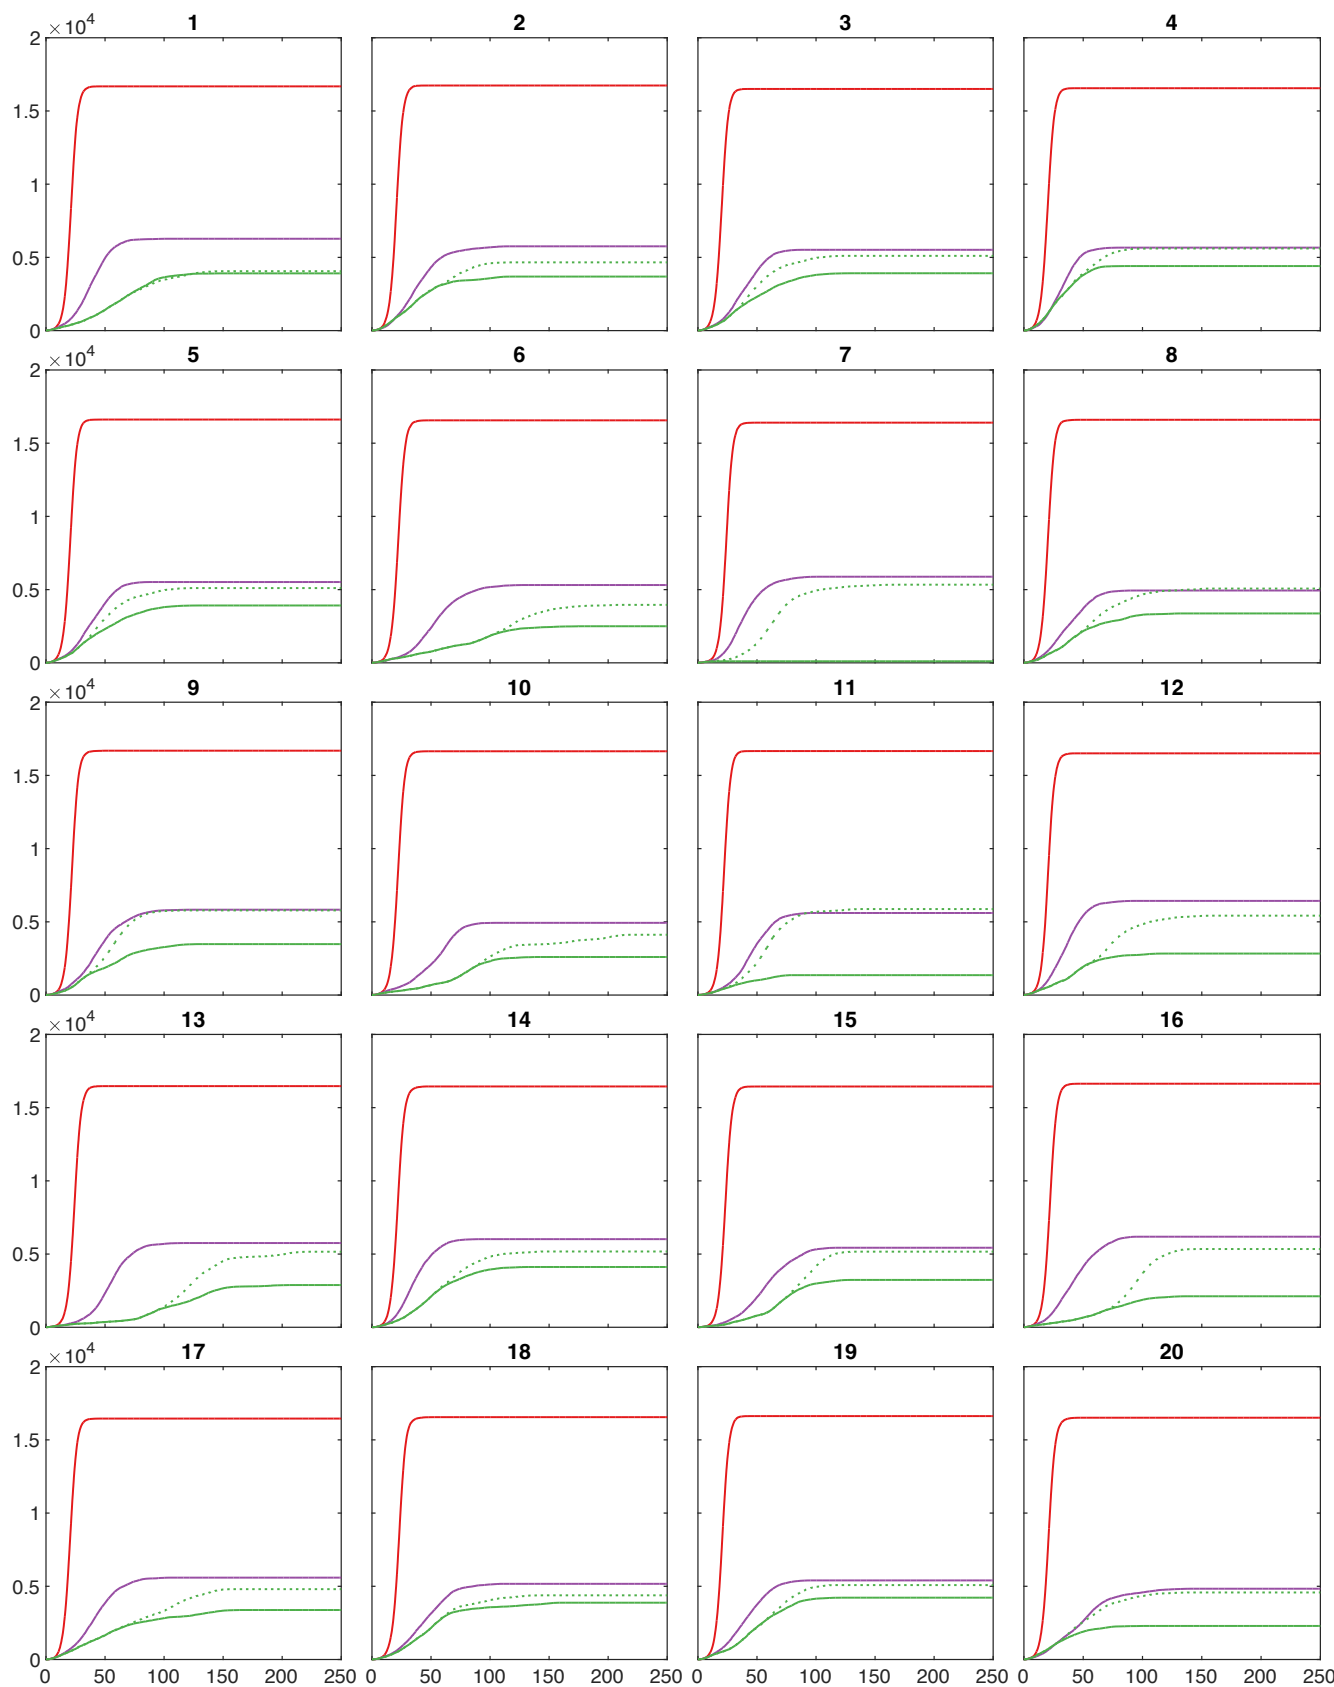

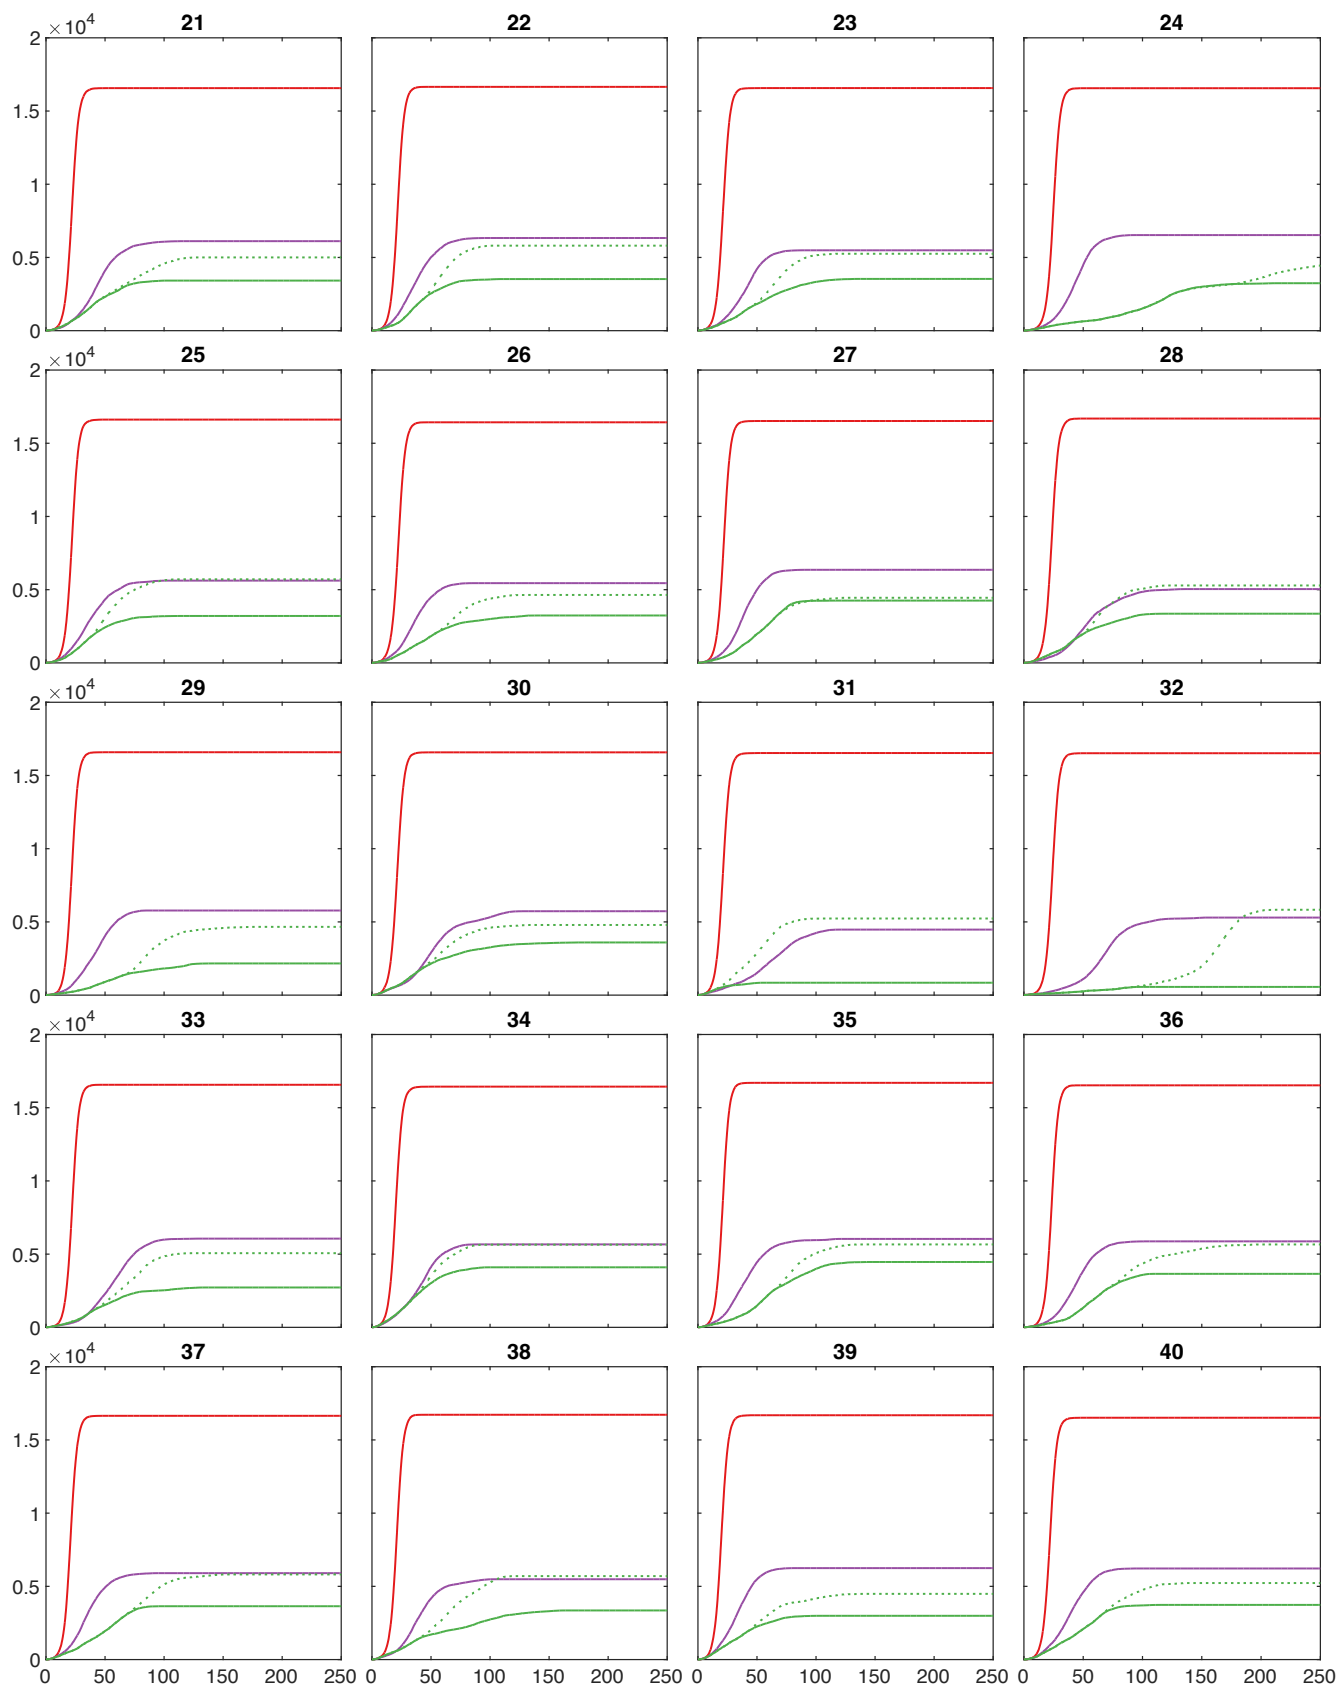

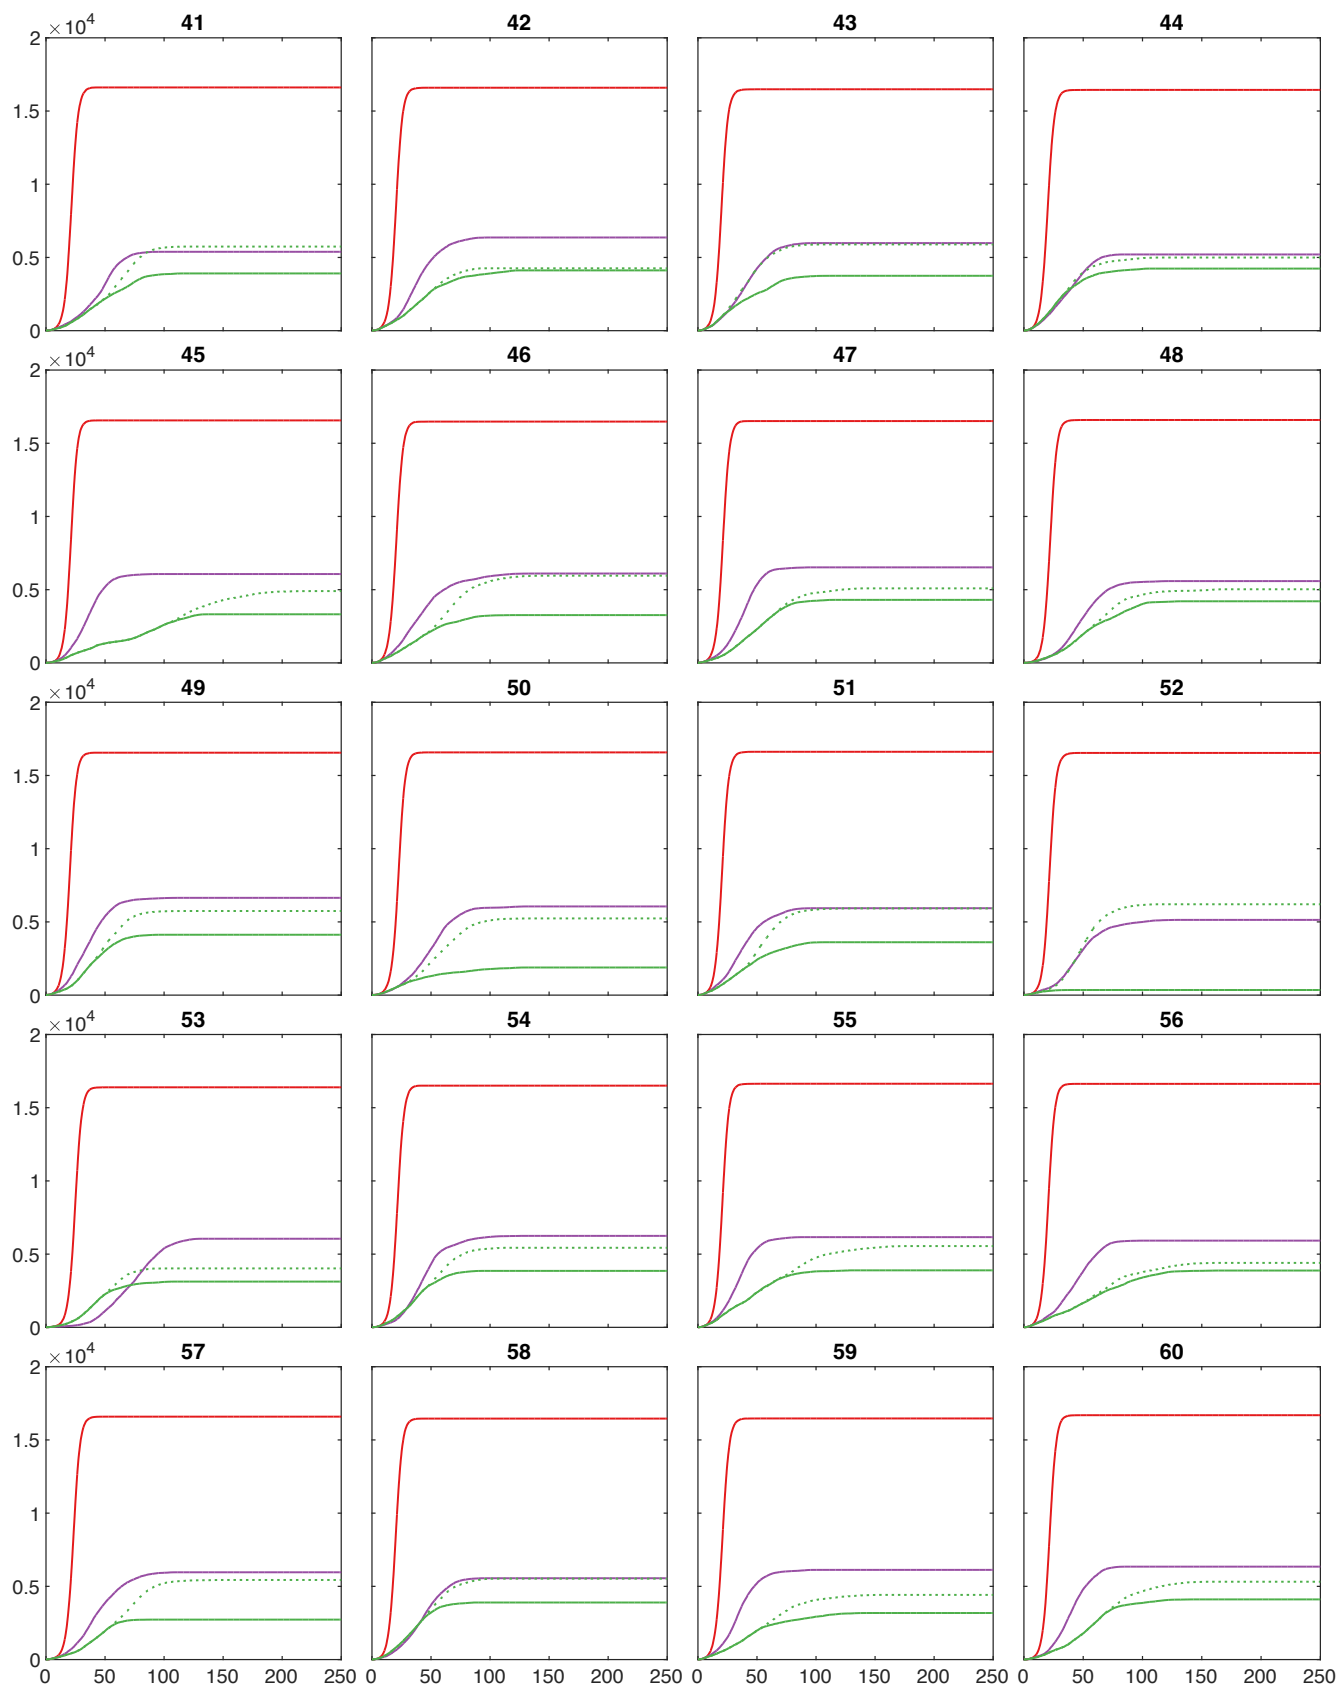

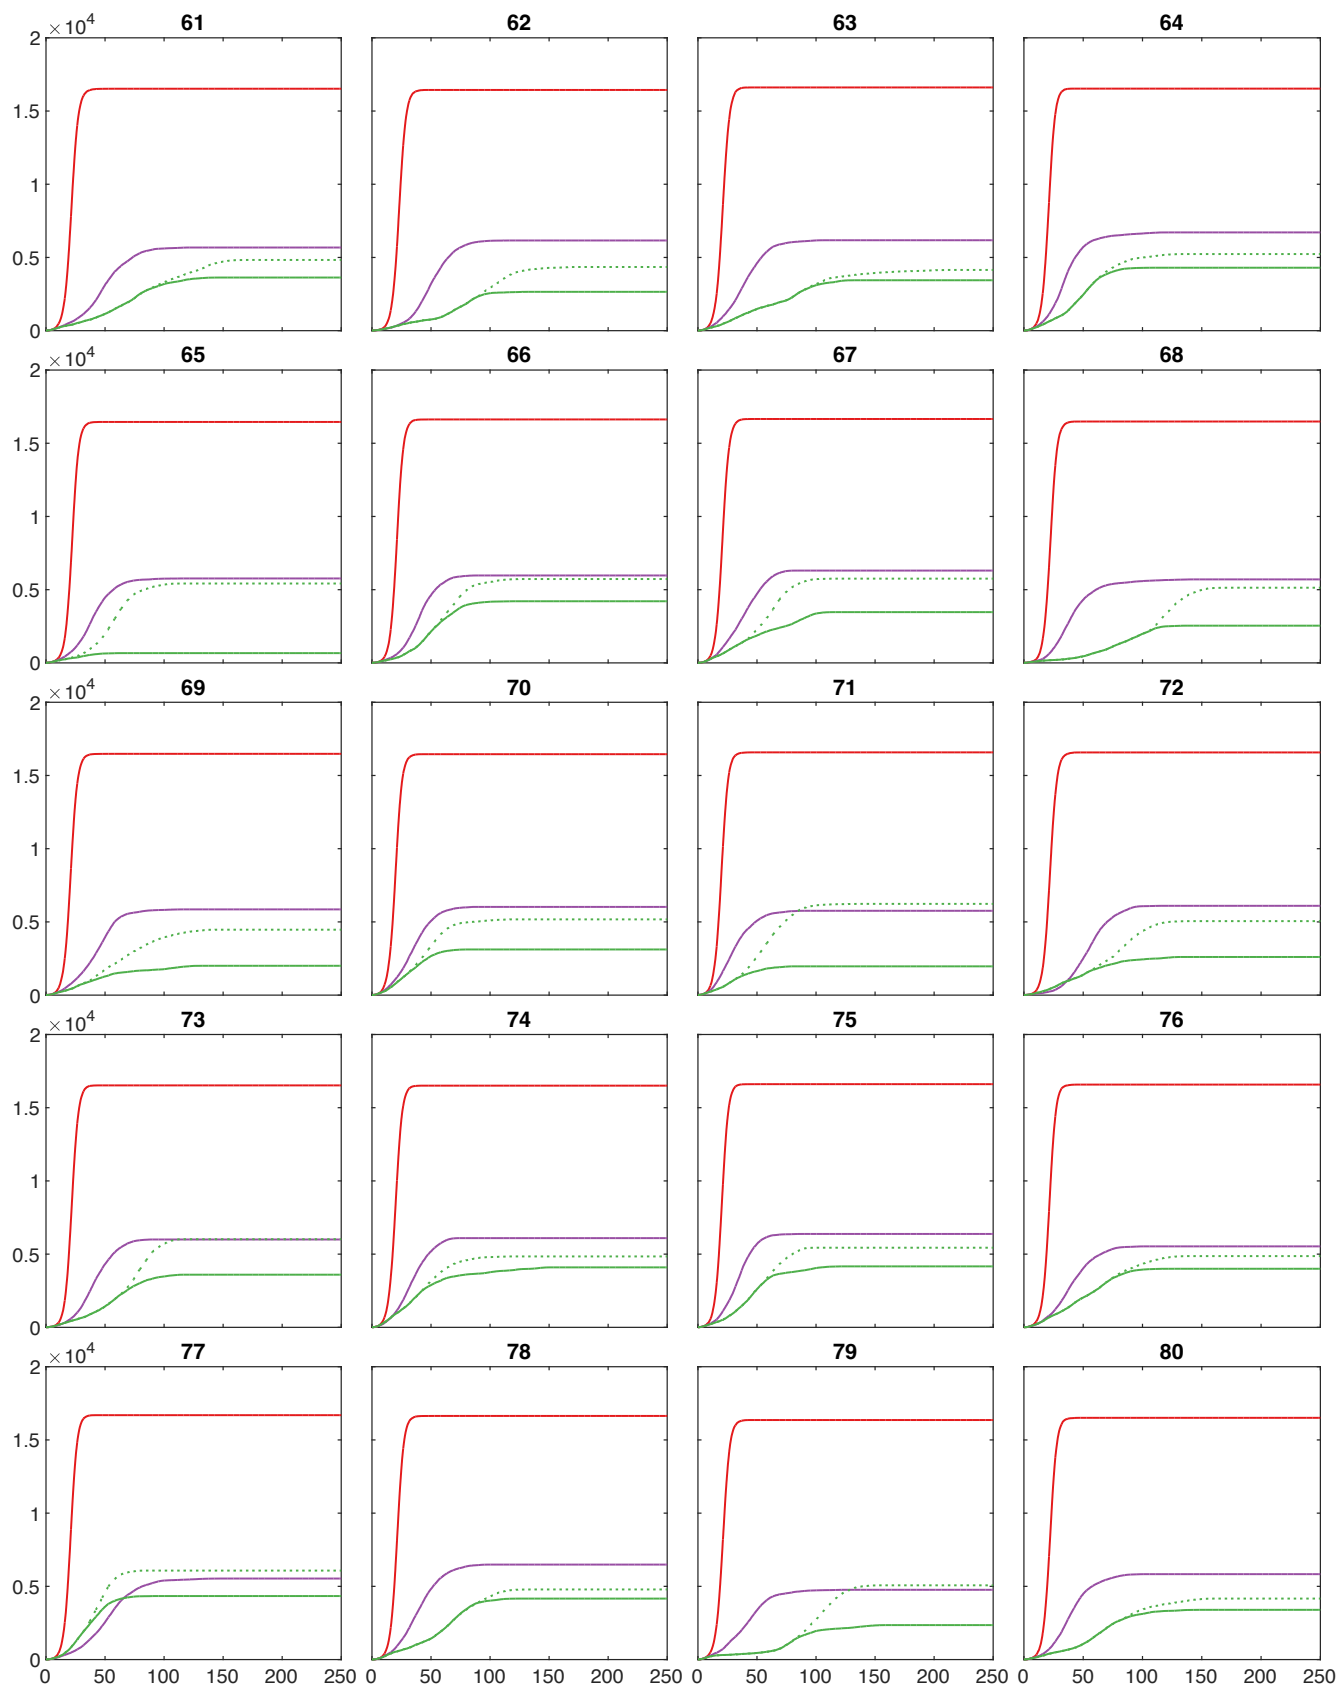



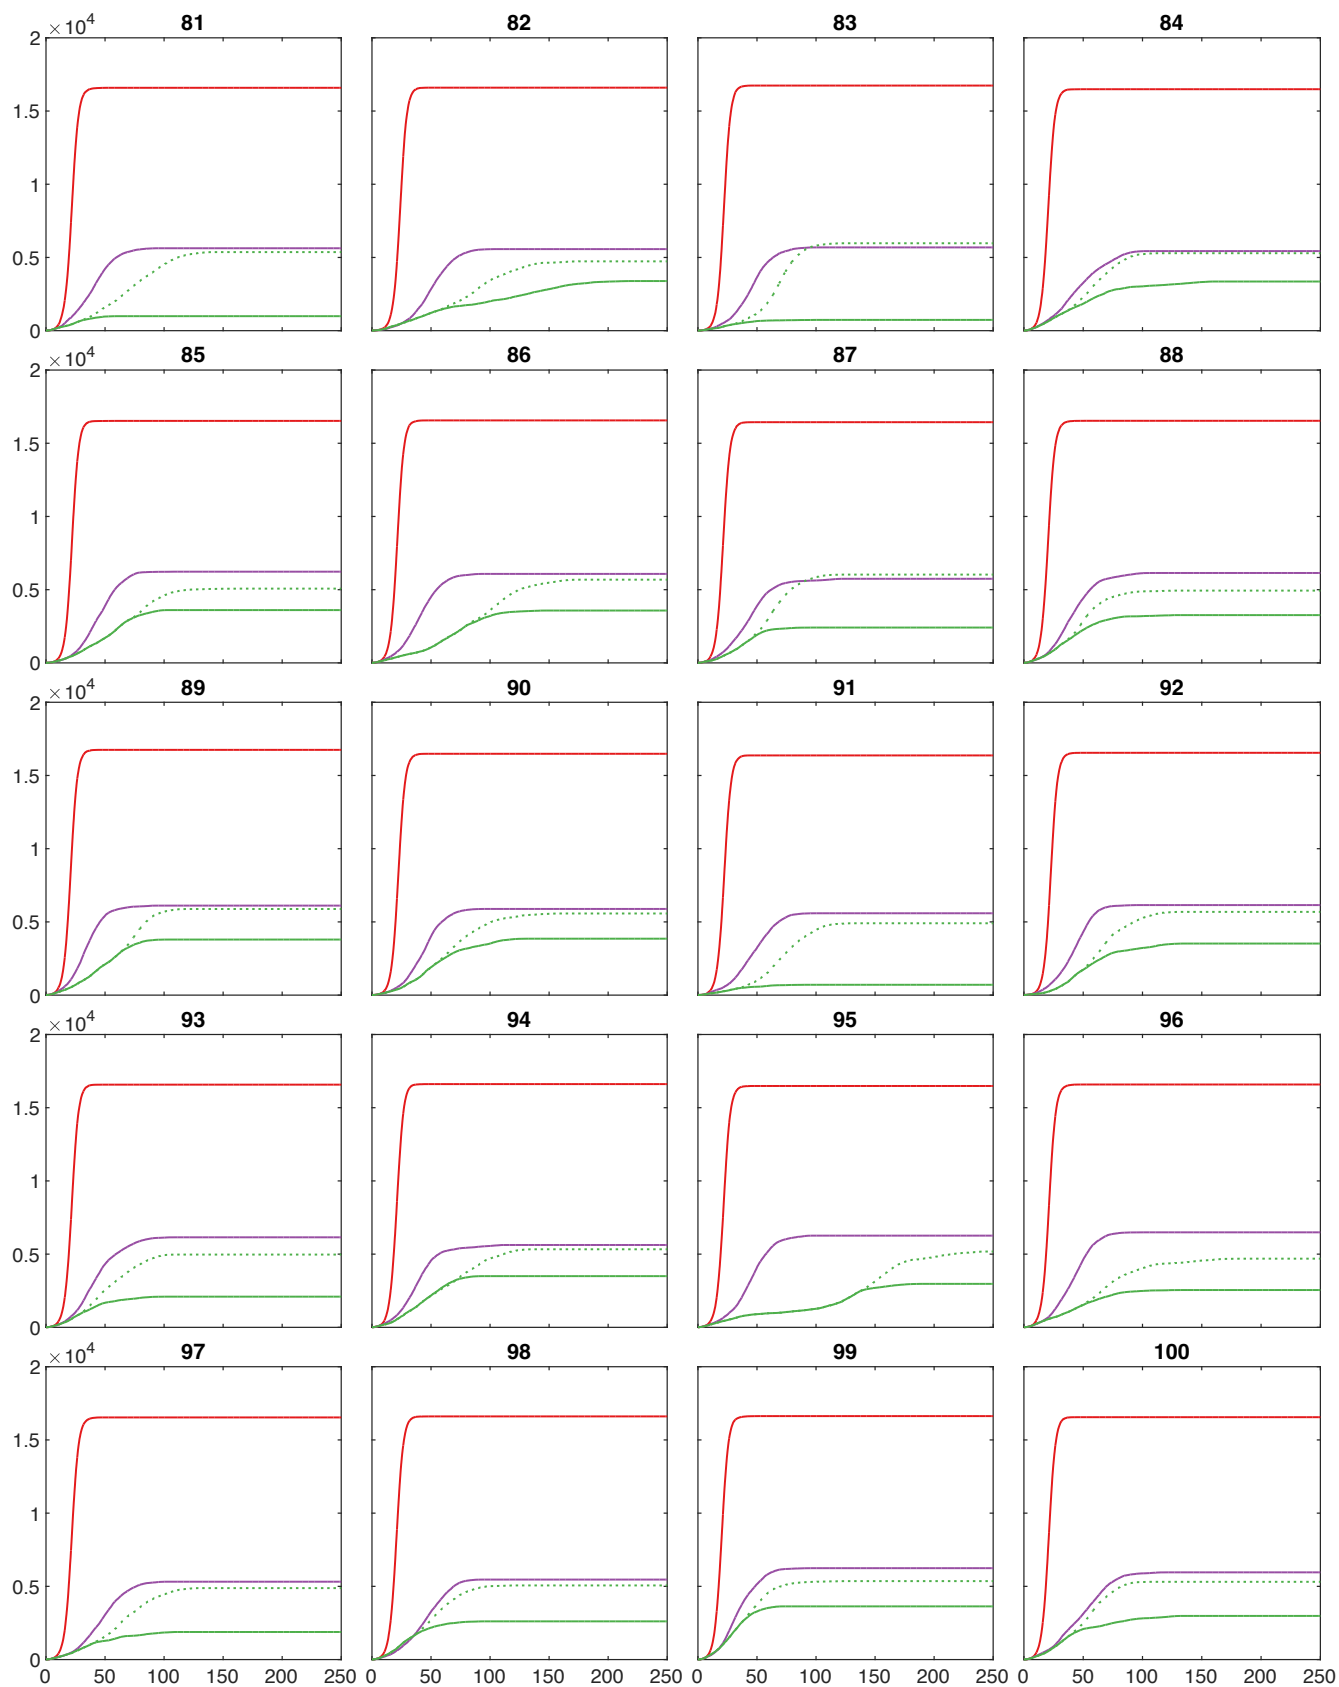

**Cumulative infection curves for all 100 simulations under the single test scenario**

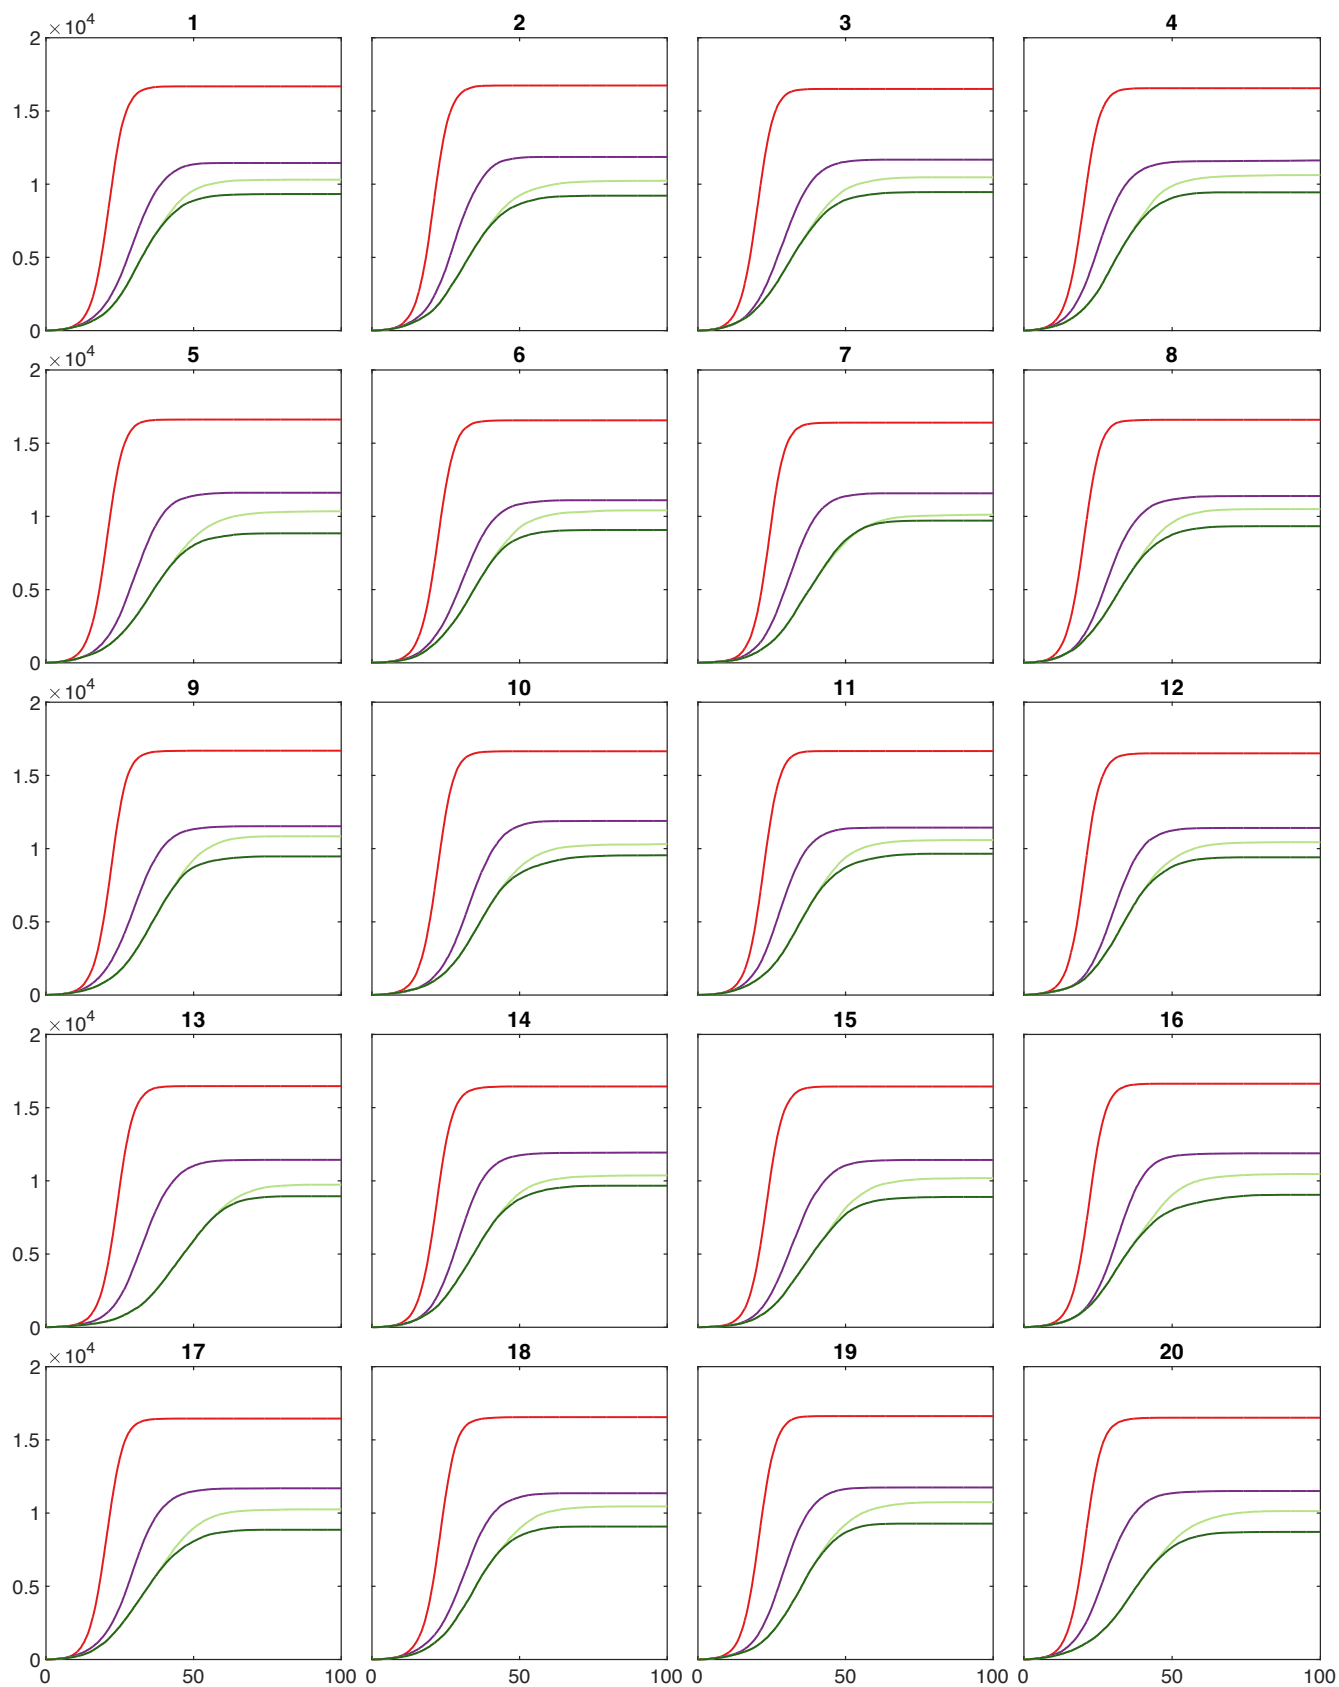

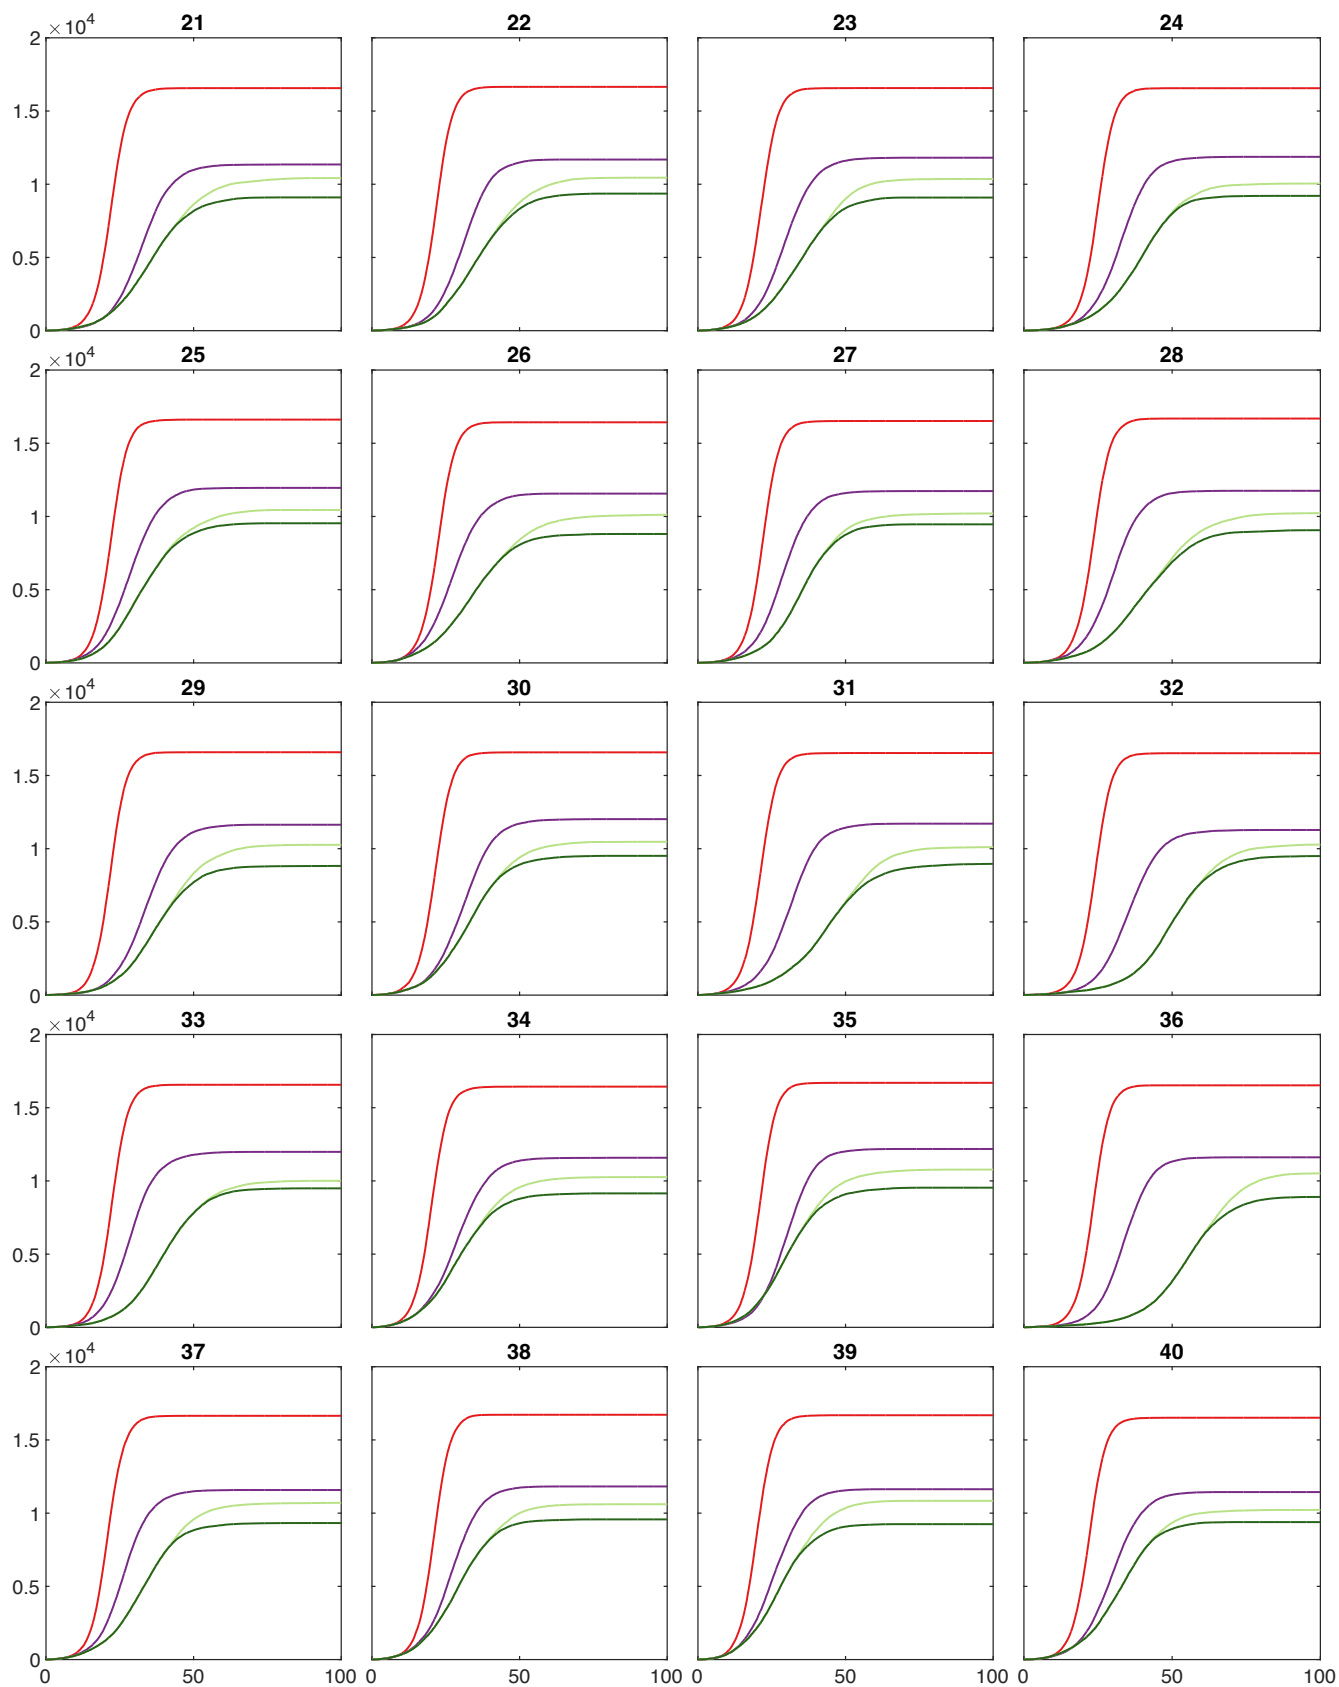

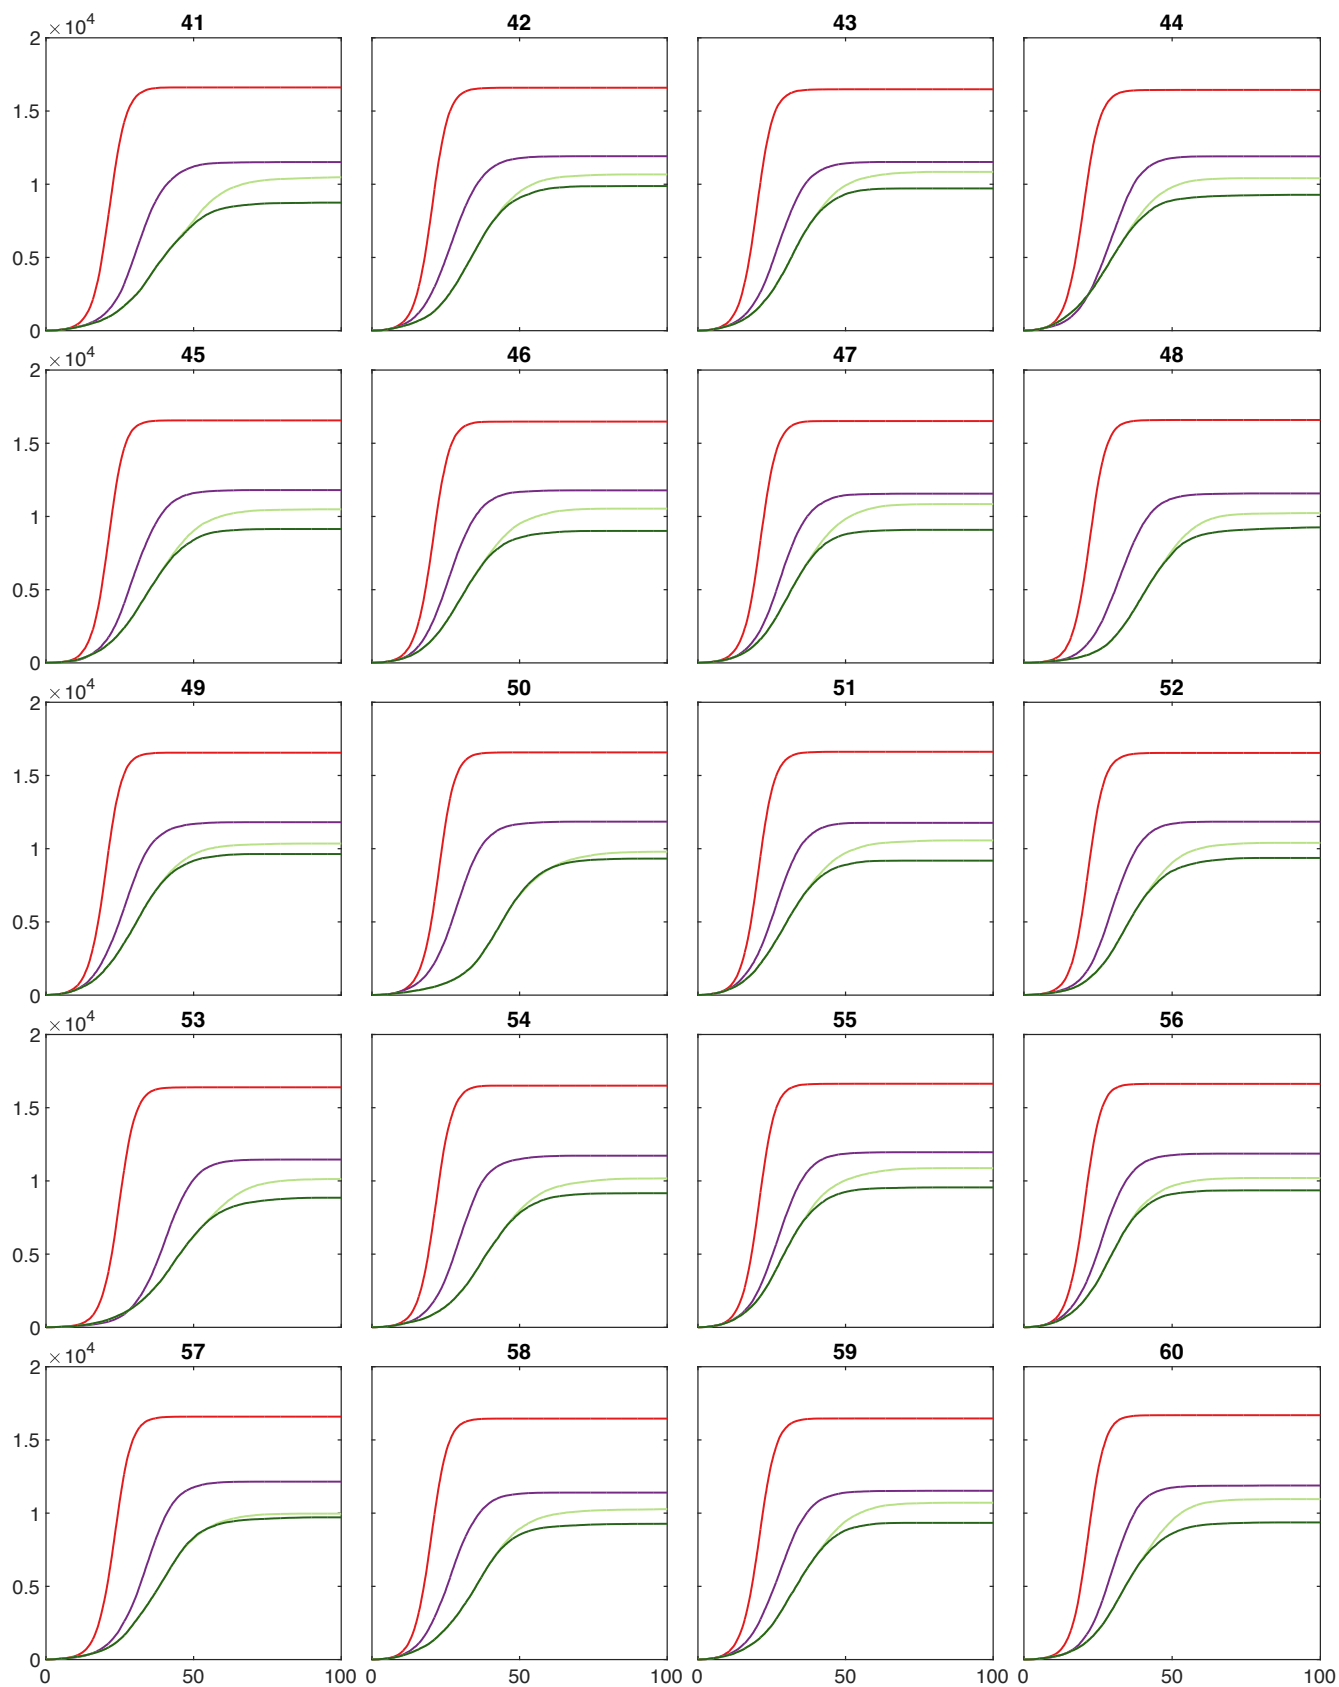

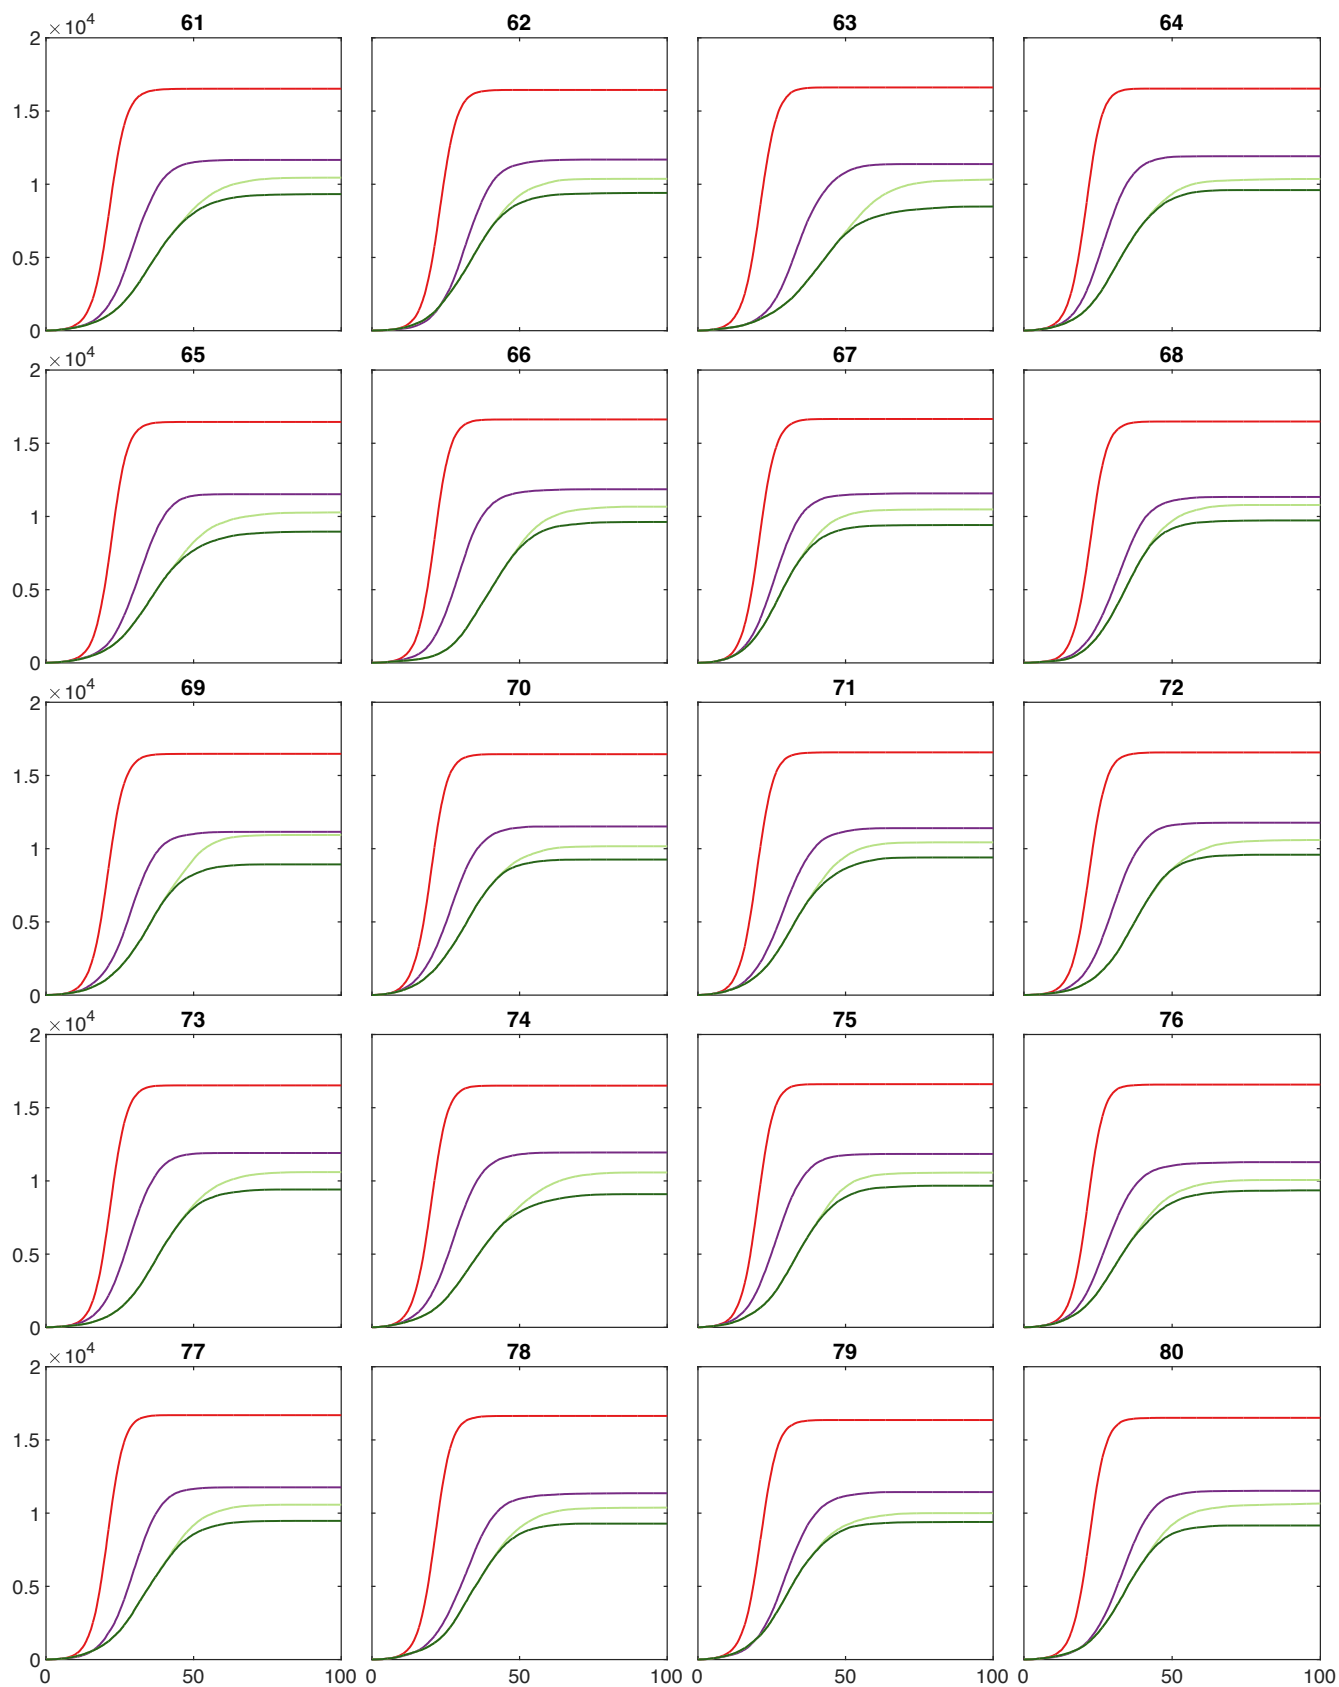

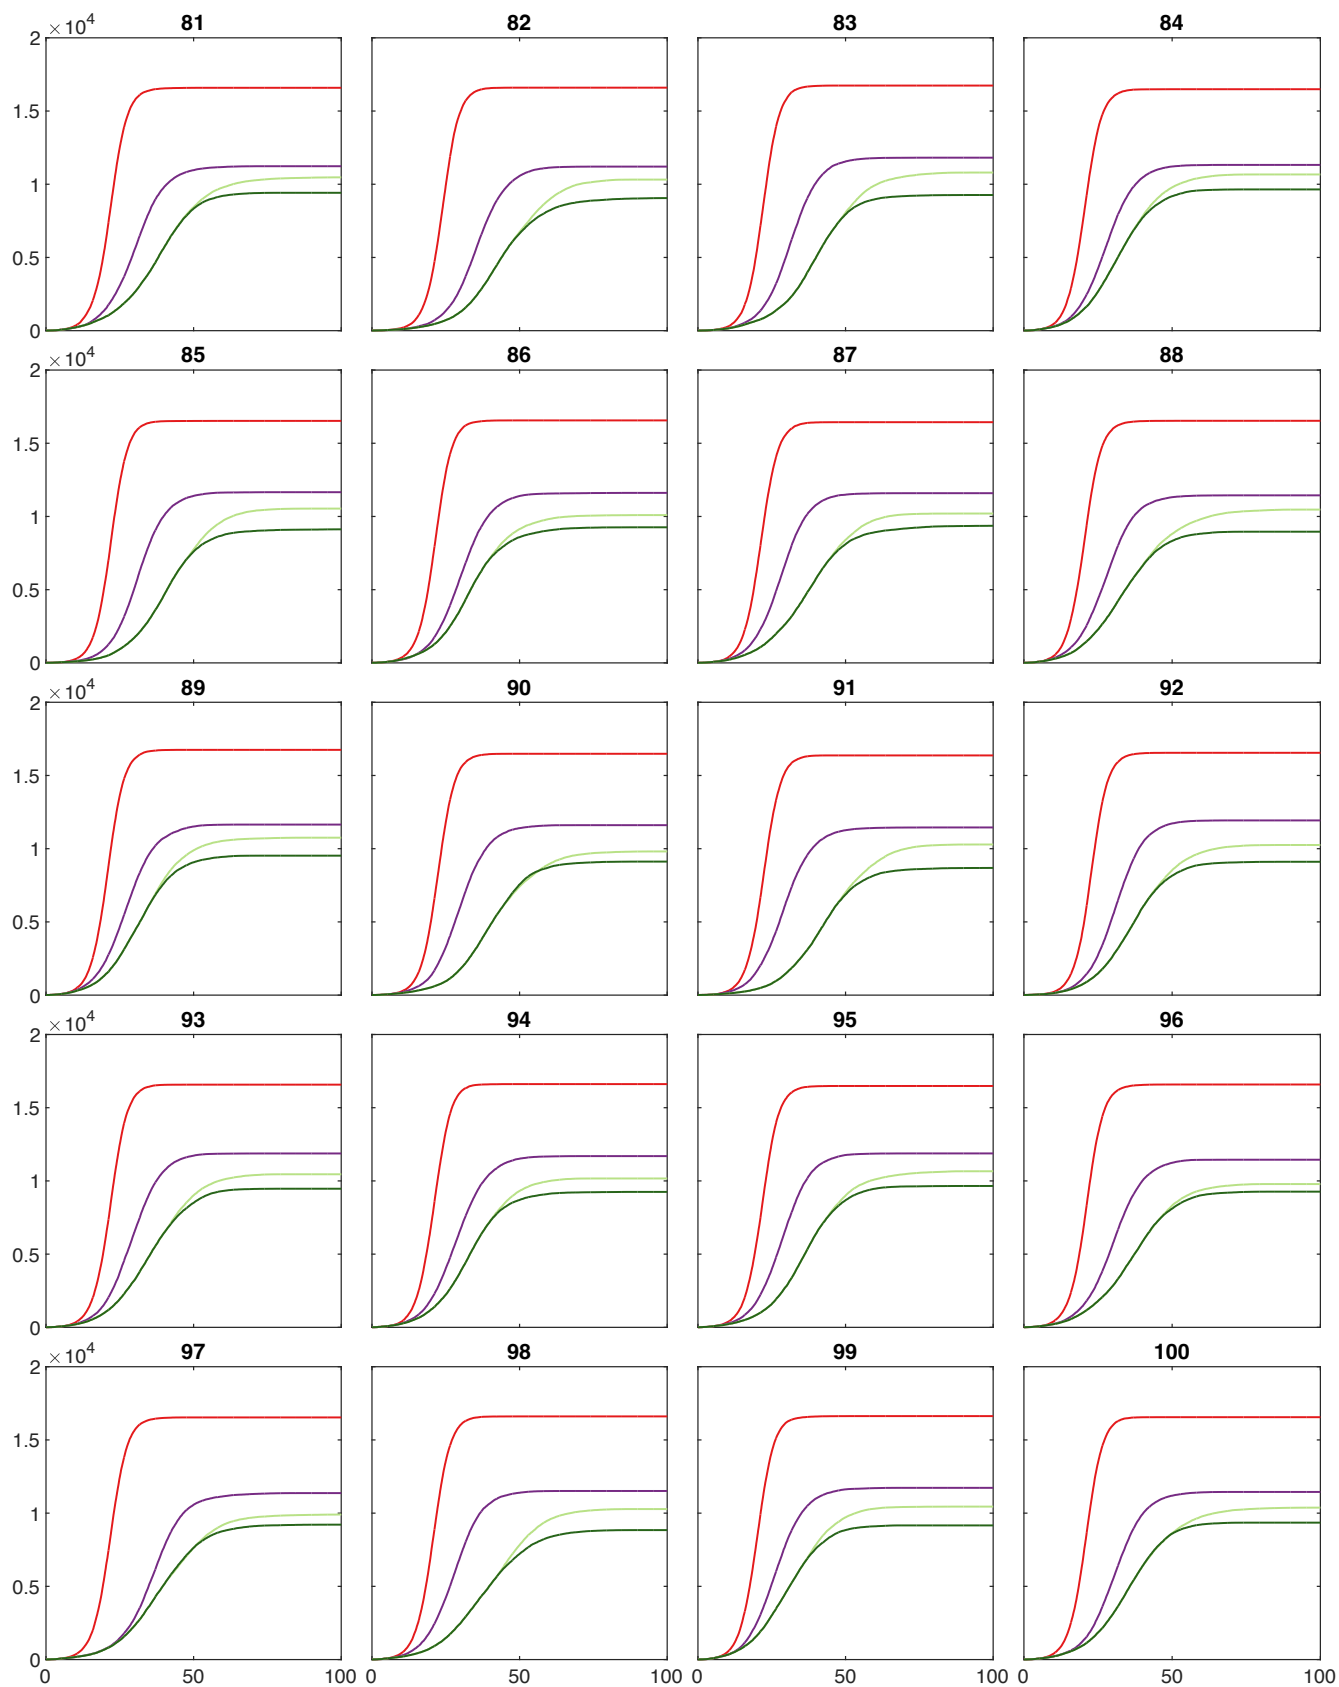

Supplement: Supplementary file 1 [file S1_Appendix.pdf]
