# Supplementary material for: Should public health policy exempt cases with low viral load from isolation during an epidemic?: a modelling study
Source: arXiv:2412.17428 source file (2025-01-31)
Supplement: Supplementary file 2 [file S2_Appendix.pdf]

## S2 Appendix

### Testing probability and test sensitivity for the 'SARS-CoV-2 like' simulations.

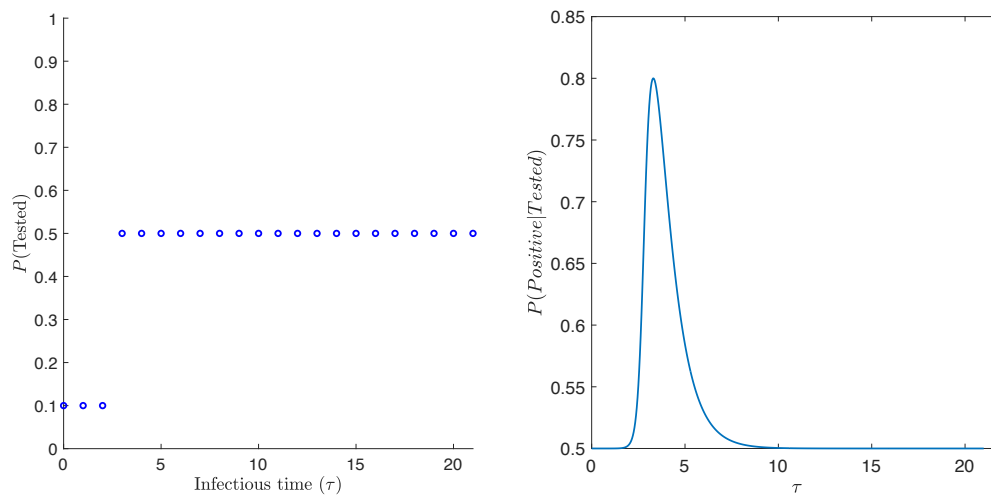

### Results with slower 'SARS-CoV-2 like' viral kinetics.

#### Multiple tests

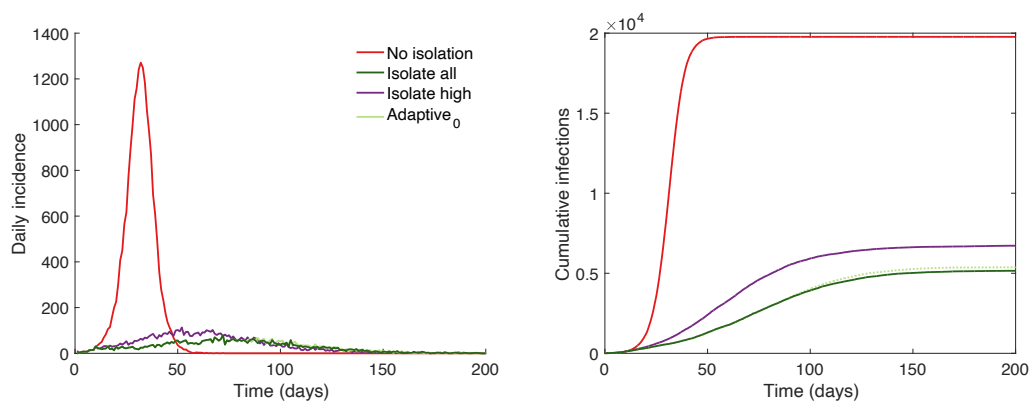

#### Single test

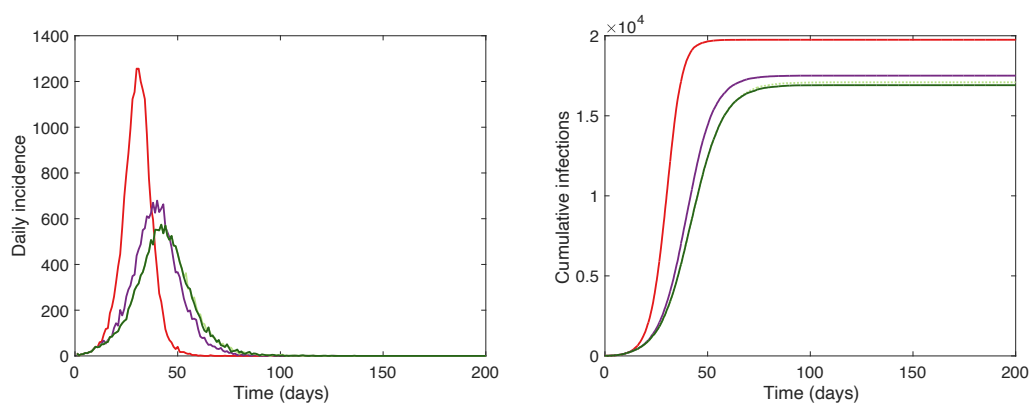

### Relative effectiveness and efficiency for the 'SARS-CoV-2 like' simulations

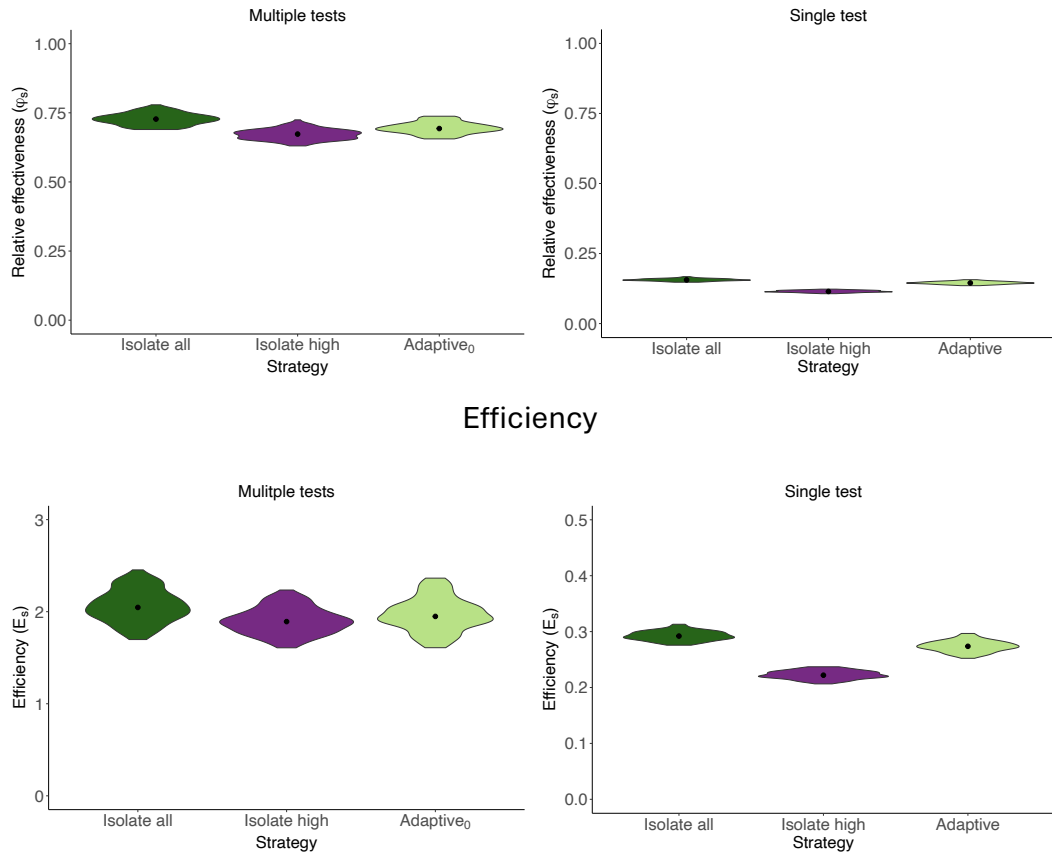

**Table of parameters and values for the ‘SARS-CoV-2 like’ simulations.**

| Parameters         | Description                                            | Value and unit                                                               | Reference           |
|--------------------|--------------------------------------------------------|------------------------------------------------------------------------------|---------------------|
| TIV model          |                                                        |                                                                              | <a href="#">[1]</a> |
| $T_k(0)$           | initial number of target cells                         | $4 \times 10^8$ cells                                                        |                     |
| $\alpha$           | rate of infection of target cells by virus             | $4.7 \times 10^{-8} [(\text{TCID}_{50}/\text{ml})^{-1} \cdot \text{d}^{-1}]$ |                     |
| $\delta_L$         | death rate of infected cells                           | $1.07 \text{ d}^{-1}$                                                        |                     |
| $p$                | rate of increase of viral titer per infected cell      | $3.07 [(\text{TCID}_{50}/\text{ml})^{-1} \cdot \text{d}^{-1}]$               |                     |
| $c$                | viral clearance rate                                   | $2.4 \text{ d}^{-1}$                                                         |                     |
| Between-host model |                                                        |                                                                              | Refer to text       |
| $\beta_{\max}$     | maximum contagiousness of the infected agents          | 0.3                                                                          |                     |
| $V_{50}$           | the viral load at which contagiousness is half maximal | $10^3 (\text{TCID}_{50}/\text{ml})$                                          |                     |
| $\xi$              | the steepness from low to high contagiousness          | 2                                                                            |                     |
| $\epsilon$         | threshold to resign agent from infected to removed     | $10^{-2} (\text{TCID}_{50}/\text{ml})$                                       |                     |
| $N$                | total population size                                  | 20000                                                                        |                     |
| $I(0)$             | initial number of infected agents                      | 10                                                                           |                     |
| $\lambda$          | average number of contacts of an infected agent        | $1 \text{ d}^{-1}$                                                           |                     |
| $t_{\text{int}}$   | time step                                              | 1 hr                                                                         |                     |

**Table 2.** Parameters and values for Covid-like agent-based model.

[1] Baccam, P., Beauchemin, C., Macken, C. A., Hayden, F. G., & Perelson, A. S. (2006). Kinetics of influenza A virus infection in humans. *Journal of Virology*, 80(15), 7590-7599.
